# Supplementary material for: LPSNet: End-to-End Human Pose and Shape Estimation with Lensless Imaging
Source: arXiv:2404.01941 source file (2024-04-08)
Supplement: Supplementary file 1 [file X_suppl.tex]

% \clearpage
% \setcounter{page}{1}
% \maketitlesupplementary
% \noindent In this document, we provide the following supplementary contents:
% % 

% \begin{itemize}
% \item Training Loss;
% \item Experimental results on simulated data;
% \item Additional Real dataset;
% \item Failure Cases and Limatations.
% \end{itemize}

% \section{Rationale}
% \label{sec:rationale}
% 
\thispagestyle{empty}
\pagestyle{empty}
\noindent In this document, we provide the following supplementary contents:
\begin{itemize}
\item Training Loss;
\item Evaluation;
\item Experimental Results on Simulated Dataset;
\item Failure Cases and Limitations.
\end{itemize}

\noindent We also provide a demo video on our \href{https://cic.tju.edu.cn/faculty/likun/projects/LPSNet}{project page}.
% 
% To split the supplementary pages from the main paper, you can use \href{https://support.apple.com/en-ca/guide/preview/prvw11793/mac#:~:text=Delete%20a%20page%20from%20a,or%20choose%20Edit%20%3E%20Delete).}{Preview (on macOS)}, \href{https://www.adobe.com/acrobat/how-to/delete-pages-from-pdf.html#:~:text=Choose%20%E2%80%9CTools%E2%80%9D%20%3E%20%E2%80%9COrganize,or%20pages%20from%20the%20file.}{Adobe Acrobat} (on all OSs), as well as \href{https://superuser.com/questions/517986/is-it-possible-to-delete-some-pages-of-a-pdf-document}{command line tools}.

\section{Training Loss}

We introduce multiple training losses as supervision for LPSNet: the reconstruction loss, the Kullback-Leibler divergence loss, and the environmental constraint loss.   Formally, the entire training loss is formulated as follows:
\begin{equation}
\mathcal{L}= \mathcal{L}_{\text {reg }}+ \mathcal{L}_{\text {das }}.
\end{equation}

\begin{itemize}   
  \item 
  \textbf{Regressor Loss $\mathcal{L}_{\text {reg }}$.}
  This loss is formulated as:
  \begin{equation}
    \mathcal{L}_{\text {reg }}=\lambda_{\text {2D }} \mathcal{L}_{\text {2D }}+\lambda_{\text {3D }} \mathcal{L}_{\text {3D }}+\lambda_{\text {para }} \mathcal{L}_{\text {para }},
    \end{equation}
    where $\mathcal{L}_{\text {2D }}$, $\mathcal{L}_{\text {2D }}$ and $\lambda_{\text {para }} \mathcal{L}_{\text {para }}$ denote the 2D keypoints loss, the 3D keypoints loss and the SMPL parameter reconstruction loss, respectively.

    \item
   \textbf{Double-Head Auxiliary Supervision Loss $\mathcal{L}_{\text {das }}$.}
    This loss is formulated as:
    \begin{equation}
    \mathcal{L}_{\text {das }}=\mathcal{L}_{\text {sc }}+ \mathcal{L}_{\text {den }},
    \end{equation}
    where $\mathcal{L}_{\text {sc }}$ and $\mathcal{L}_{\text {den }}$ denote the IUV   Supervision loss and Keypoints Supervision loss:
    \begin{equation}
    \begin{aligned}
    \mathcal{L}_{sc} =\lambda_{x y} \left(\operatorname{KL-Loss}({x} , \hat{x}) + \operatorname{KL-Loss}({y} , \hat{y})\right),
    \end{aligned}
    \end{equation}

    \begin{equation}
    \begin{aligned}
    \mathcal{L}_{den} & =\lambda_{p i} \text { CrossEntropy }(P, \hat{P}) \\
    & +\lambda_{u v} \operatorname{SmoothL1}( U,  \hat{U}) \\
    & +\lambda_{u v} \operatorname{SmoothL1}( V, \hat{V}). \\
    % & +\lambda_{u v} \operatorname{SmoothL1}(\hat{P} \odot V, \hat{P} \odot \hat{V}) \\
    \end{aligned}
    \end{equation}

\end{itemize}

\section{Evaluation Metrics}
Here, we describe the evaluation metrics we used in our experiments.
First, we report the widely used MPJPE (mean per joint position error), which is calculated as the mean of the Euclidean distances between the ground truth and the predicted joint positions after centering the pelvis joint on the ground truth location (as is common practice):
\begin{equation}
MPJPE=\frac{1}{N} \sum_{i=1}^N\left\|p_i-q_i\right\|_2 .
\end{equation}
Also, we report PA-MPJPE (Procrustes Aligned MPJPE), which is calculated similarly to MPJPE but after a rigid alignment of the predicted pose to the ground truth pose,
\begin{equation}
P A-M P J P E=\frac{1}{N} \sum_{i=1}^N\left\|p_i-q_i\right\|_2 .
\end{equation}
Furthermore, we calculate Per-Vertex-Error (PVE), which is denoted by the Euclidean distance between the ground truth and predicted mesh vertices that are the output of SMPL layer:
\begin{equation}
P VE=\frac{1}{M} \sum_{j=1}^M\left\|v_j-w_j\right\|_2 .
\end{equation}

% \section{Additional Real dataset}
% The additional real dataset is mainly captured by a lensless imaging system we fabricated for real human body information, and we also use Inertial measurement unit(IMU) to record human pose information.
\begin{figure}[h]
  \centering
  % \fbox{\rule{0pt}{2in} \rule{0.9\linewidth}{0pt}}
   \includegraphics[width=0.95\linewidth]{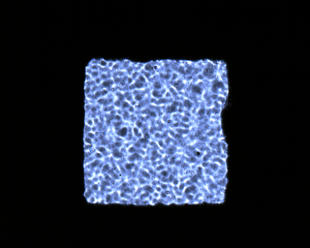}

   \caption{The PSF acquired by our imaging system.}
   \label{fig6}
\end{figure}

\section{Experimental Results on Simulated Dataset}
We also create a simulation dataset; through the simulation dataset, the feasibility of our experiment can be further verified. 
We create a simulation application based on the principle of lensless imaging to model the imaging process of lensless imaging.
We design the simulation application by referring to the imaging model of PhlatCam~\cite{boominathan2020phlatcam}.
A real-world 2D scene $\mathbf{i} (x, y; z)$ at a distance z can be assumed to be made up of incoherent point sources. Each point source will produce a shifted version of PSF $p_z (x, y)$, and since the sources are incoherent to each other, the shifted PSF will add linearly in intensity~\cite{goodman2005introduction}  at the sensor.
By Property 1 of the PSF, we can write the imaging model as the following convolution model:
\begin{equation}
\mathbf{b} (x, y)=p_z (x, y) * \mathbf{i} (x, y ; z).
\end{equation}
Here, b is the sensor’s capture, and \text { * } denotes 2D convolution over $(x, y)$.
We capture the PSF of our system as shown in ~\cref{fig6}, and we use the PSF and the existing human posture dataset to get the simulation dataset based on the imaging modality.
We perform simulations on the Human3.6M dataset~\cite{ionescu2013human3}.
~\cref{fig1} and ~\cref{fig2} show the results of LPSNet on the simulated dataset.

\section{Failure Cases and Limatations}
There are some limitations and some difficult cases that we have not solved very well. ~\cref{fig5}, ~\cref{fig3}, ~\cref{fig4} shows, some failure cases of our approach. When human movement is more complex, the human pose and shape, as estimated by LPSNet, will have a large deviation.
As shown in ~\cref{fig3}, the error in human pose and shape estimation also becomes larger when the human body proper is obscured.

\begin{figure}[h]
  \centering
  % \fbox{\rule{0pt}{2in} \rule{0.9\linewidth}{0pt}}
   \includegraphics[width=0.95\linewidth]{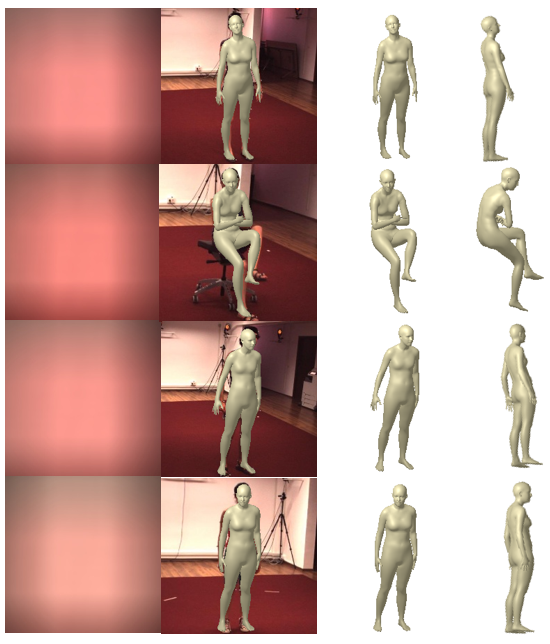}

   \caption{
   From left to right: lensless measurements, alignment of the estimated body mesh with the original scene, and reconstruction results of LPSNet on the simulated dataset.}
   \label{fig1}
\end{figure}

\begin{figure}[t]
  \centering
  % \vspace{-12cm}
  % \fbox{\rule{0pt}{2in} \rule{0.9\linewidth}{0pt}}
   \includegraphics[width=0.95\linewidth]{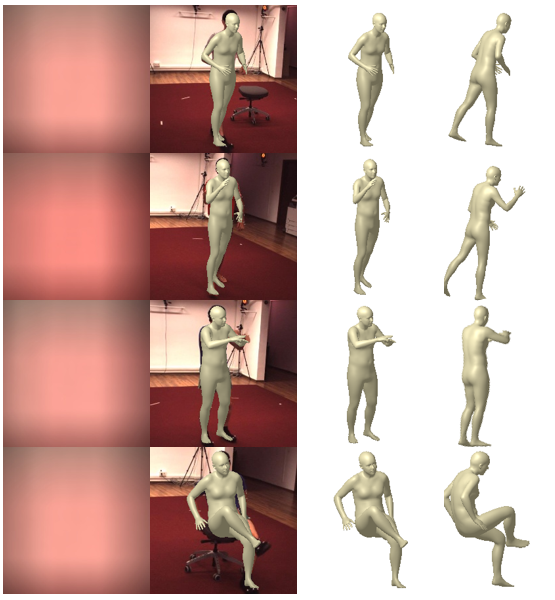}

   \caption{From left to right: lensless measurements, alignment of the estimated body mesh with the original scene, reconstruction results of LPSNet on the simulated dataset.}
   \label{fig2}
\end{figure}
% \section{Real Scene}
% \begin{figure}[h]
%   \centering
%   % \fbox{\rule{0pt}{2in} \rule{0.9\linewidth}{0pt}}
%    \includegraphics[width=0.8\linewidth]{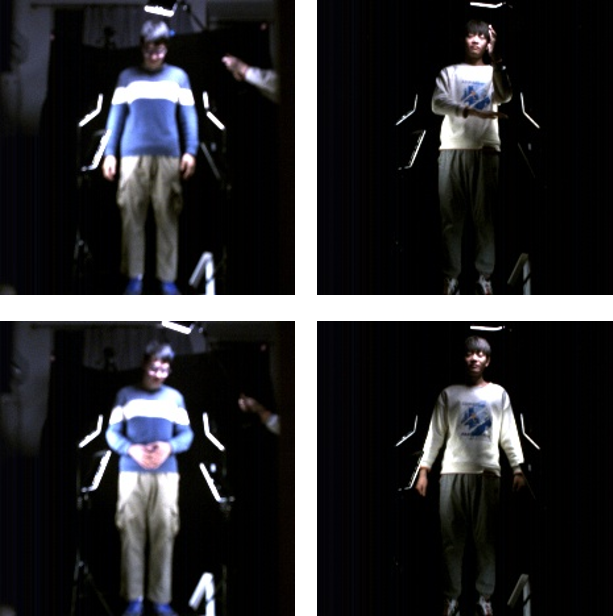}

%    \caption{These given images represent a real scene. There are two different characters, one on the left and one on the right.
%    }
%    \label{fig:4.1.2}
% \end{figure}

\begin{figure*}[h]
  \centering
  % \fbox{\rule{0pt}{2in} \rule{0.9\linewidth}{0pt}}
   \includegraphics[width=0.95\linewidth]{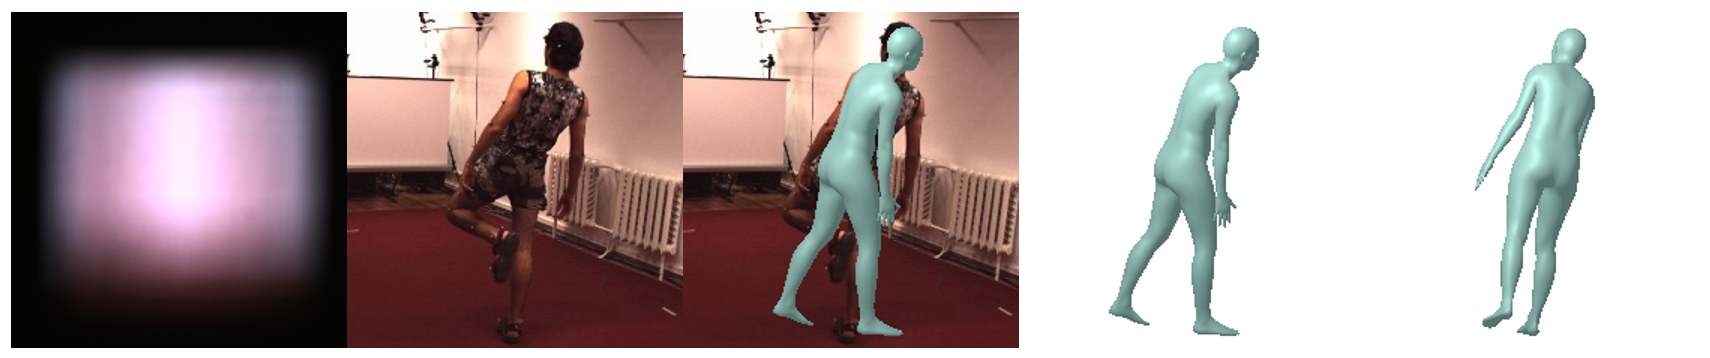}

   \caption{\textbf{Failure results for LPSNet.} From left to right: lensless measurements, real scene, alignment of the estimated body mesh with the original scene, reconstruction results of LPSNet. The poses of the characters in the scene are more complex and difficult to reconstruct.}
   \label{fig5}
\end{figure*}
\begin{figure*}[h]
  \centering
  % \fbox{\rule{0pt}{2in} \rule{0.9\linewidth}{0pt}}
   \includegraphics[width=0.95\linewidth]{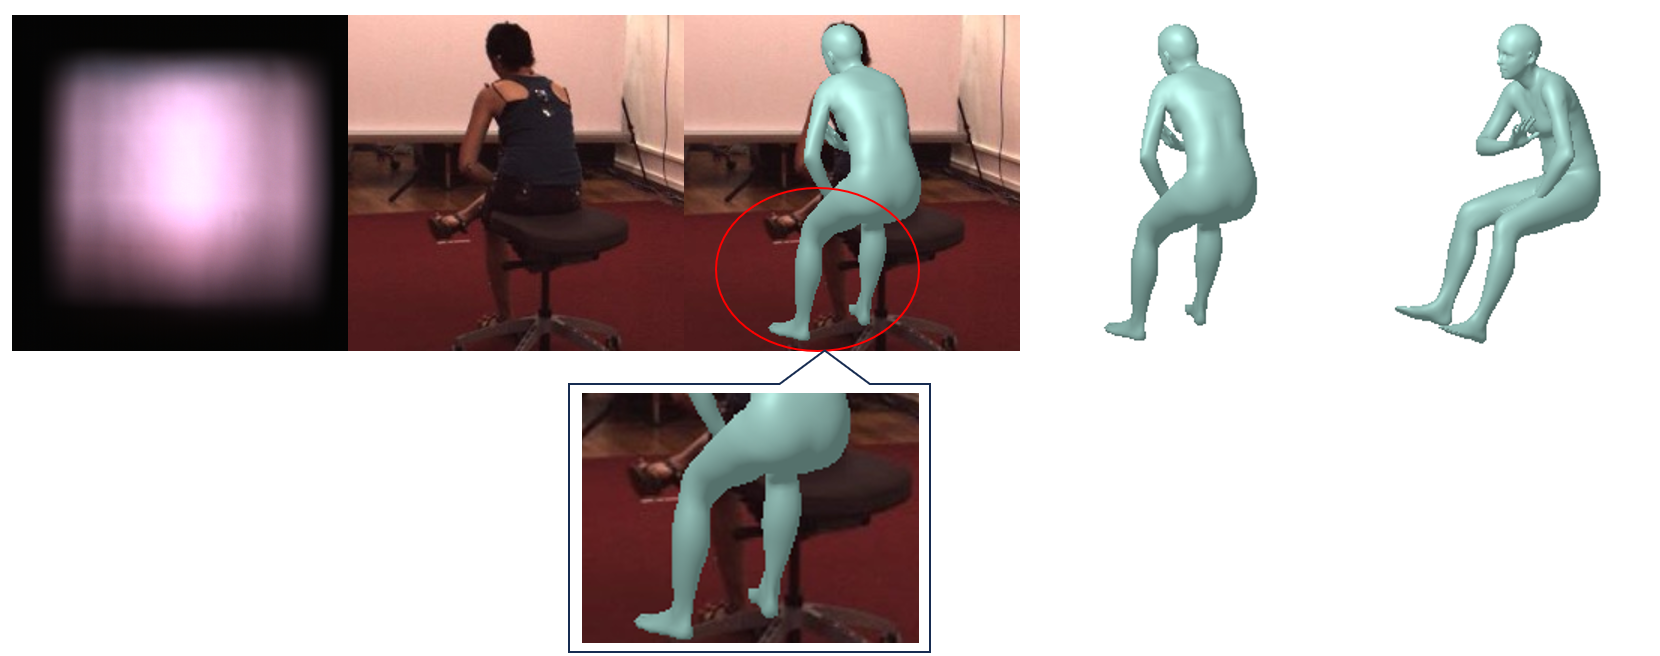}

   \caption{\textbf{Failure results for LPSNet.} From left to right: lensless measurements, real scene, alignment of the estimated body mesh with the original scene, reconstruction results of LPSNet. The enlarged image shows that the reconstruction of the obscured part fails.}
   \label{fig3}
\end{figure*}

\begin{figure*}[h]
  \centering
  % \fbox{\rule{0pt}{2in} \rule{0.9\linewidth}{0pt}}
   \includegraphics[width=0.95\linewidth]{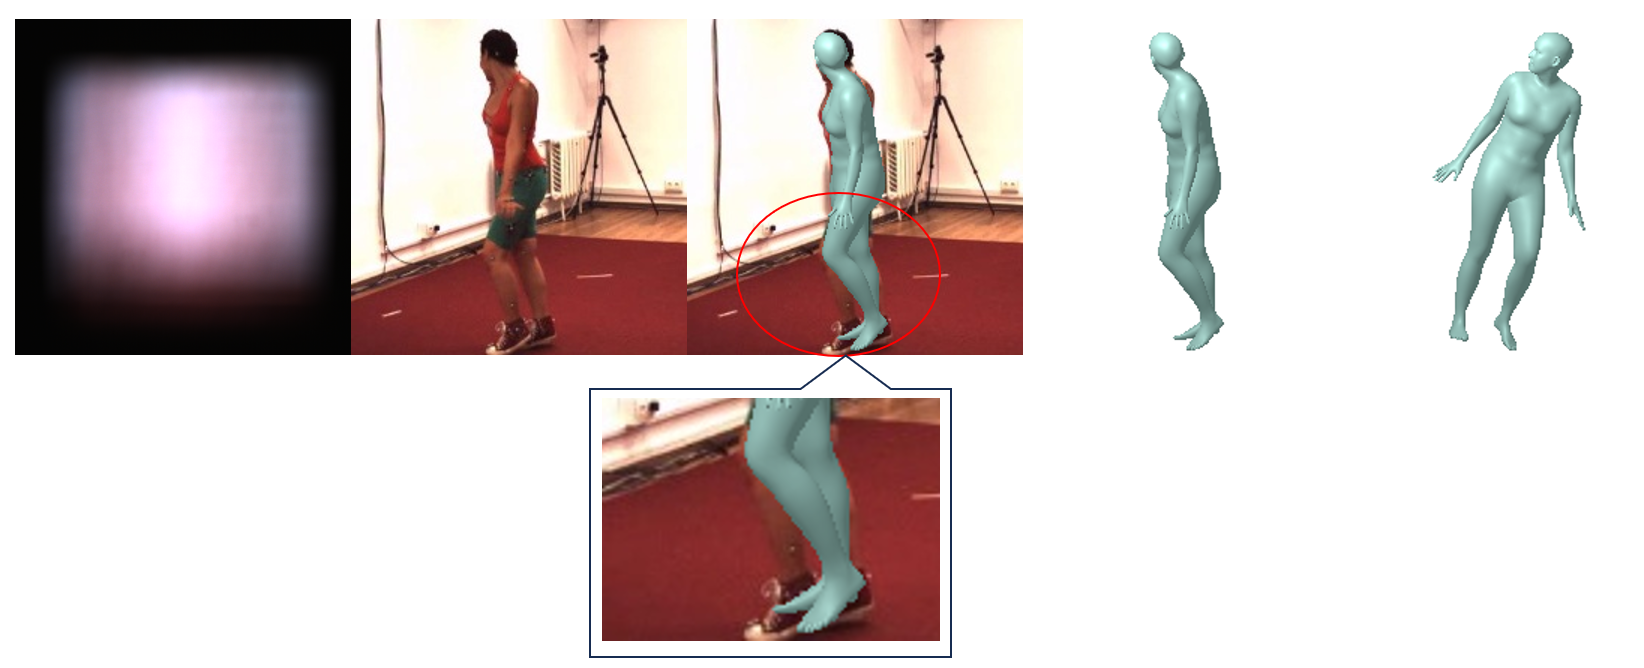}

   \caption{\textbf{Failure results for LPSNet.} From left to right: lensless measurements, real scene, alignment of the estimated body mesh with the original scene, reconstruction results of LPSNet. Poses overlap heavily with large reconstruction errors.}
   \label{fig4}
\end{figure*}

\clearpage
